# Supplementary material for: NoiseBench: Benchmarking the Impact of Real Label Noise on Named Entity Recognition
Source: arXiv:2405.07609 source file (2024-10-14)
Supplement: Supplementary file 1 [file ablation_rt.tex]

\section{Ablation: Sentiment Classification}

In addition to NER, which is the main focus of this paper, we also investigate how noise-robust approaches perform in the sentiment classification task when faced with real label noise. 

\subsection{Dataset} This task is represented by the Rotten Tomatoes Movie Reviews (\rottentomatoes) dataset \cite{pang-lee-2005-seeing}, which includes sentences extracted from online movie reviews aimed for binary classification based on whether the sentiment is positive or negative. We follow the methodology for the creation of \benchmark{} and create clean training and test splits, as well as 4 additional variants of the training set, labeled with different types of noise. The training set consists of 5000 examples from the \rottentomatoes~dataset, for which \citet{rodrigues2013learning} have published crowdsourced labels. Since the full \rottentomatoes~dataset contains 10000 examples, we include the remaining 5000 data points as our clean test set. We create 4 noisy variants of the training split: \noisecrowdbest, \noisecrowd, \noiseweak~and \noisellm \ in the same way as those in \benchmark{}. The resulting noise shares are shown in the first row in Table \ref{exp3_rt_results}. %, together with the summarized results of noise-robust methods are shown in Table 

% % , with their noise levels shown in Table \ref{conll_noise_shares_table}. For this task, we express the noise levels in terms of error rate, as a percentage ($100 - \%Accuracy$).

\subsection{Experimental setup}
We repeat the evaluation of noise-robust approaches on the sentiment classification task. As a baseline, we fine-tune an \texttt{xlm-roberta-large} transformer. % with the same parameters. 
In addition to the baseline, we again evaluate three noise-robust approaches, and provide the same theoretical upper bounds. 

\textbf{Noise-robust approaches.} Same as for NER, we evaluate Confident learning and Co-regularization for this task, however since BOND is a NER-specific approach, we evaluate another conceptually similar approach \textbf{COSINE} \citep{yu2021fine}. It is also a two-stage approach that follows a regular transformer fine-tuning objective in the first step (on weak labels), and a contrastive self-training objective to suppress label noise propagation afterwards. The self-training stage also relies on the high-confidence samples in order to update the model. Similarly to BOND, we stop the first stage manually after the 4th epoch, and limit the second stage to 6 epochs. We perform a small hyperparameter search in order to find the optimal ones for each noise type, as suggested by the authors.

\begin{table*}[]
\centering
\small
\setlength{\tabcolsep}{4pt}
\begin{tabular}{p{3cm} r r r r r r r r}
\toprule
 & \noiseclean & \noisecrowdbest & \noisecrowd & \noiseweak & \noisellm & Average \tabularnewline \midrule
\%Noise & - & 8.9 & 11.0 & 44.5 & 12.1 & - \tabularnewline \midrule
Baseline & 89.28{\scriptsize±0.07} & 88.79{\scriptsize±0.12} & 88.07{\scriptsize±0.22} & 65.45{\scriptsize±1.02} & 86.43{\scriptsize±0.09} & 83.60 \tabularnewline  \midrule
 \multicolumn{3}{l}{\textit{Upper bounds}} & & & & & & \tabularnewline
Oracle subset & - & 89.42{\scriptsize±0.09} & 89.13{\scriptsize±0.11} & 87.70{\scriptsize±0.32} & 88.45{\scriptsize±0.27} & \textbf{88.68}  \tabularnewline
Oracle stopping & 89.43 {\scriptsize±0.20} & 88.81{\scriptsize±0.07} & 88.42{\scriptsize±0.06} & 70.45{\scriptsize±2.98} & 87.19{\scriptsize±0.16} &  84.86\tabularnewline 
\midrule
 \multicolumn{3}{l}{\textit{Noise-robust learning}} & & & & & &  \tabularnewline
Co-regularization & \textbf{89.76}{\scriptsize±0.15} & \textbf{89.36}{\scriptsize±0.24} & \textbf{88.92}{\scriptsize±0.14} & \textbf{72.21}{\scriptsize±2.00} & \textbf{87.94}{\scriptsize±0.17} & 85.64 \tabularnewline
Confident learning &88.93{\scriptsize±0.16} & 88.59{\scriptsize±0.07} & 88.00{\scriptsize±0.09} & 72.03{\scriptsize±0.48} & 86.94{\scriptsize±0.19} & 84.90 \tabularnewline
COSINE & 88.83{\scriptsize±0.36} & 88.48{\scriptsize±0.44} & 88.62{\scriptsize±0.16} & 61.50{\scriptsize±10.18} & 86.92{\scriptsize±0.08} & 82.87 \tabularnewline 
%\midrule \multicolumn{3}{l}{\textit{zero-shot}} & & & & & & \tabularnewline LLM & 87.82 & & & & & & \tabularnewline
\bottomrule
\end{tabular}
\caption{\label{exp3_rt_results} Performance of noise-robust approaches on the Clean RT-MR test set, when training on \benchmark{} label sets. Results are expressed in terms of Accuracy score. Each score is averaged over 3 runs.}
\end{table*}

% The Rotten Tomatoes subset (the Sentiment benchmark) is split randomly, with 20\% of the sentences being included in the validation set.
% As a classification metric we calculate accuracy

\subsection{Results}

The results from this ablation experiment are presented in Table \ref{exp3_rt_results}.

\textbf{Noise share.} Regarding the noise shares of different types of noise, we can note that they are rather low in comparison to the corresponding \benchmark \ label sets, except for the Weak label set. This indicates that real label noise can have varying degrees of difficulty depending on the task.

\textbf{Noise robustness.}
 We can see that Co-regularization is a clear winner among the noise-robust learning approaches. Once again, the baseline is outperformed only slightly, but in this case, the theoretical upper bound is not that far away from the baseline, except for the Weak label set.

Furthermore, the \noiseclean~label set here actually probably corresponds to the \noiseexpert~label set of \benchmark, since there were no re-labeling efforts made when it comes to the Rotten Tomatoes dataset%, or any of the popular sentiment classification datasets for that matter
. This can explain why the \noisecrowdbest~upper bound is higher than the \noiseclean~baseline.

This ablation highlights the advantages of \benchmark, for evaluating future noise-robust approaches. It allows for a range of realistic noisy label sets with varying noise shares, and as a result levels of difficulty, while providing a high-quality clean test set. In addition, \benchmark~ represents a generally harder, but much less ambiguous task.

% cosine doesn't work because we are not using it right - Weak reduced to MV, with a lot of random labels, which COSINE first takes only the subset which is covered.

% indicates that the Rotten Tomatoes task is a relatively easy task, since the discrepancy between the baseline and Oracle subset results is quite small for almost all noise types. 

% Other points:

% 1. Noise shares low, even LLM, excluding Weak with very high noise (almost random labels). Crowd labels around 10\% noise, unlike for NER. For this problem the relationship between different noise sources and their levels is different. 

% 2. All oracle subsets are very close to Clean baseline, meaning much fewer samples are needed to achieve .89 or close to it

% 3. would also mention that LLM noise share is 12 (we can also maybe  add that we got the same number on the test set), which is very close to 89 and looks like fine-tuning doesn't help much. %Easy (few clean samples,...) to get to 87 (even zero-shot LLM does it), but almost impossible to get over 90 (the task is not hard, but probably many ambiguous samples which are impossible to get right). 

% 4. Takeaway: This ablation showcases that realistic noise can have varying degrees of difficulty, depending on the task???

% 5. 'Clean' set is in fact expert (no relabelling rounds like in conll). Reason why Crowd++ upper bound is higher than clean.

% maybe try to frame this setup as a "bad" benchmark for evaluating noise robustness. benefits of NoiseBench for NER: range of noise shares, harder task, high quality clean data available...
