# Supplementary material for: NoiseBench: Benchmarking the Impact of Real Label Noise on Named Entity Recognition
Source: arXiv:2405.07609 source file (2024-10-14)
Supplement: Supplementary file 2 [file appendix_analysis_of_predictions_baseline.tex]

\section{Extended Performance Metrics}
\label{sec:appendix-test-errors}

In this section we provide extended metrics of the predictive performance of the baseline FLERT method. 

\subsection{Generalization to Unseen Entities}
\label{appendix:seen_vs_unseen}

\input{figures/seen_vs_unseen_plots}

We evaluate the generalization of the baseline model from Experiment 1 (Section \ref{Exp1}) by calculating F1 scores for seen and unseen entities separately, and further distinguishing seen entities according to whether their label in the training set was clean or noise-corrupted. On Figure \ref{fig:seen_vs_unseen_real} we observe that for the \noiseexpert~and \noisecrowdbest~noise types, the performance for the seen (clean) entities and the unseen entities is comparable, which indicates the model has the ability to generalize to unseen entities well. The overall drop in performance when training with these noisy training splits is largely due to the low performance on the seen (noisy) entities. However, this detrimental effect of memorization is limited to the seen errors and does not affect the performance on unseen entities much, for noise levels up to 15\%. As for the remaining training splits with noise levels of 30\% and above, we can see that noise affects the performance on unseen entities as well.
Furthermore, on Figure \ref{fig:seen_vs_unseen_simulated}, we see that for simulated noise, for \noiseexpert~and \noisecrowdbest~, the performance on seen noisy entities is close to the performance on seen clean entities. This means that at low noise levels, the models are able to disregard the noisy patterns and predict the same entities correctly when they appear in the test set, instead of memorizing the noisy label. 

% why is the model hurt by Expert so much? I think it's because CleanCoNLL consistently cleans some types of noise

\input{additional_content/appendix_per_class_metrics}

\input{additional_content/appendix_test_error_types}
