# Supplementary material for: NoiseBench: Benchmarking the Impact of Real Label Noise on Named Entity Recognition
Source: arXiv:2405.07609 source file (2024-10-14)
Supplement: Supplementary file 3 [file appendix_simulated_noise_overview.tex]

\section{Overview of simulated datasets}
\label{sec:appendix-simulated-noise-extended}

In this section we provide an extended overview of the simulated noisy datasets. 

We can see that simulated noise has much fewer type errors and more missing mentions, wrong mentions and partial matches. This again shows that other than in terms of token-level F1, the real and simulated noise are not similar in terms of the shares of different types of errors they include.

\begin{table*}[]
\centering
\small
\setlength{\tabcolsep}{4pt}
\begin{tabular}{@{}lrrrrrrrrrrr@{}}
\toprule
 &  & & & & & \multicolumn{2}{c}{\textit{\#Entities}} &\multicolumn{4}{c}{\textit{\#Errors}} \\
 \cmidrule(lr){7-8}  \cmidrule(lr){9-12}  
& \textit{\%Noise} & \textit{F1}\scriptsize{token} & \textit{F1} & \textit{Prec.} & \textit{Rec.} & \textit{\#Entities} & \textit{\#Correct} & \textit{Missing (FN)} & \textit{Mention (FP)} & \textit{Type} & \textit{Partial} \\ \midrule
\textit{Training splits} &  &  &  &  &  &  &  &  &  &  &  \\
\noiseclean & 0 & 100 & 100 & 100 & 100 & 9,685 & 9,685 & 0 & 0 & 0 & 0 \\
\noiseexpert & 5.9 & 99 & 94.5 & 94.7 & 94.3 & 9,680 & 9,114 & 210 & 205 & 361 & 112 \\
\noisecrowdbest & 17.9 & 96 & 82.1 & 86.8 & 77.8 & 8,686 & 7,537 & 1,854 & 855 & 294 & 530 \\
\noisecrowd & 41.3 & 91.2 & 58.7 & 68.5 & 51.4 & 7,278 & 4,982 & 4,048 & 1,641 & 655 & 912 \\
\noisedistant & 39.2 & 92.2 & 60.8 & 69.7 & 53.9 & 7,496 & 5,224 & 3,961 & 1,772 & 500 & 1,103 \\
\noiseweak & 41.2 & 91.8 & 58.8 & 55.7 & 62.2 & 10,814 & 6,023 & 1,995 & 3,124 & 1,667 & 795 \\
\noisellm & 47.2 & 88.8 & 52.8 & 48.3 & 58.1 & 11,640 & 5,626 & 2,256 & 4,211 & 1,803 & 419 \\
\bottomrule
\end{tabular}
\caption{\label{conll_noise_shares_table_simulated} (Simulated noise) Overview of the training and test splits in \benchmark. The table shows the noise level, the micro-averaged token-level F1 score (\textit{F1}\begin{scriptsize} token\end{scriptsize}), micro-averaged entity-level F1 (\textit{F1}), precision (\textit{Prec.}), recall (\textit{Rec.}); as well as number of entities (\textit{\#Entities}) and number of correct entities (\textit{\#Correct}). It also shows the number of incorrect entities for each type of error: missing boundaries (\textit{Missing(FN)}), incorrectly labeled mentions with a wrong boundary (\textit{Mention(FP)}) and wrong type (\textit{Type}), as well as the number of partial matches (\textit{Partial}). } 
\vspace{-2mm}
\end{table*}
